# Supplementary material for: Effective Prime Factorization via Quantum Annealing by Modular Locally-structured Embedding
Source: arXiv:2310.17574 source file (2023-10-26)
Supplement: Supplementary file 1 [file appendix.tex]

\section*{Appendix}

% \begin{itemize}
% \item different initializations
% \item excitation of CFAs vs that of chains -> take the related proposal to another paper?
% \item different chain strength
% \item symmetry embedding
% \end{itemize}

\subsection*{Exploiting thermal relaxation and reverse annealing: some insights}

We report additional details about our experiments on thermal relaxation and reverse annealing, to justify why it is better to start from lower $S_p$ values for forward annealing and higher $S_p$ values for reverse annealing. 

First, we show a brief experimental analysis to support the choice of the lowest-energy sample to perform reverse annealing with respect to the other samples. To evaluate the goodness of the initial state of reverse annealing,
we examined their Hamming distance with respect to the solution, considering the factorization problems of Table \ref{tab: thermal_fluctuations_in_FW} where a solution has been found. The results are reported \ref{fig: dist_to_gs_4_FW} and Table \ref{tab: thermal_fluctuations_in_FW}. We noticed that the minimal energy sample may not guarantee the closest distance to the global minimum; there could be other samples with higher energy values but with fewer mismatching qubits. We remark, however, that choosing a minima with a high Hamming distance from the solution (for instance, consider the minimum of energy equal to $2.0$ at pausing point $S_p=0.5$)
could make the convergence to the global minimum even harder. From these assumptions, we can state that the minima obtained by pure annealing $T_a=10\mu s$,
as shown in Table \ref{tab: minimas_of_pure_FW},
represents a good start for reverse annealing for most cases, unless a minimum closer (with respect to the Hamming distance) to the ground state exists and slightly higher energy than the lowest energy exists.

\begin{figure}[ht]
    \centering
    \includegraphics[width=.8\textwidth]{figs/updated_results/Foward annealing (Tp=100us|Ta=10us)(for 16, 17, 18 bits|dist_to_gs).png}
    \caption{\label{fig: dist_to_gs_4_FW} Distances of the minimas obtained in Table \ref{tab: thermal_fluctuations_in_FW}
    for some success cases of finding groundstates.}
\end{figure}
\begin{table}[ht]
    \scriptsize
    \begin{minipage}{.48\textwidth}
        \centering
        \begin{tabular}{l|r|r|r}
            \toprule
            bits   & inputs  & energy    & distance to groundstate   \\
            \midrule
            \multirow{3}{*}{8+8}   & 49949   & 4.0       & 115   \\
               & 52961   & 6.083     & 180   \\
               & 63001   & 2         & 125   \\
            \bottomrule
        \end{tabular}
    \end{minipage}
    \begin{minipage}{.48\textwidth}
        \centering
        \begin{tabular}{l|r|r|r}
            \toprule
            bits   & inputs  & energy    & distance to groundstate   \\
            \midrule
            \multirow{2}{*}{9+8}   & 116561  & 6.167     & 159   \\
               & 122669  & 10.167    & 183 \\
            \bottomrule
        \end{tabular}
    \end{minipage}
    \caption{\label{tab: minimas_of_pure_FW} Minimas obtained by pure foward annealing ($T_a=10\mu s$)}
\end{table}

In Figure \ref{fig: comparison_of_diff_pause_lengths_and_diff_initial_state} we report information about several batches of experiments on $10\times8$ numbers that were not factorized by the quantum local search. In particular, we consider for each value of $S_p$ different pause time, in the set of values $T_p \in \{10, 50, 100, 200\} \mu s$, reporting the data of the lowest energy sample obtained and their respective Hamming distance with respect to the ground state sample. We observe that fixed a value for pause length $T_p$, thermal relaxation affects annealing by changing more qubits (thus escaping the local minimum more frequently) if the reversion point is set to higher values. For this reason, we test the $S_p$ values in decreasing order during reverse annealing.

\begin{figure}
    \centering
    \includegraphics[width=.8\textwidth]{figs/updated_results/factoring 10+8 bits/Reverse annealing (Tp|Ta=10us) from the minima obtained from forward annealing (Tp=100us|Ta=10us).png}
    \includegraphics[width=.8\textwidth]{figs/updated_results/factoring 10+8 bits/Reverse annealing (Tp|Ta=10us) from the minima obtained from forward annealing Ta=10us).png}
    \caption{{\label{fig: comparison_of_diff_pause_lengths_and_diff_initial_state}} 
    Comparisons of different pause lengths and initial states for reverse annealing
    for factoring integers of 10+8 bits}
\end{figure}

%%%% TO PUT ON SECOND PAPER

\ignore{

\subsection*{Different chain strengths}
In main paper, we use the extended coupling range, $[-2, 1]$,
for encoding the CFA function and the strongest coupling, $c=2$, for anti-ferromagnetic chains.
Here, we show three different chain strengths for the extra-chain initialization
(without using the improved CFA penalty function)
and describe their effects in terms of 
the success probability of find satisfying assignments
and the number of samples in which no chain is broken
and the number of samples in which all CFA penalty functions work correctly,
which are shown respectively in bottom and top figures of Fig \ref{fig: diff_couplings}.
The similar experiments are done for the case 
where only original coupling range, $[-1, 1]$,
is used for encoding CFA and chain.
Note that in both encoding cases with different coupling ranges,
the minimal coupling is the lower bound of the corresponding range, 
$-2$ for the extended coupling range and $-1$ for the original coupling range.
From the obtained success probabilities, we can conclude
that the chain coupling strength brings the best performance,
if chosen the same as the minimal coupling of CFA penalty function.
Either choosing stronger or weaker than the minimal coupling of CFA penalty function for chains 
will not bring better performance, as shown by $c=1.5$ and $c=0.5$ on the right Figure.
Note that the {\it long-chain-broken issue},
that the longer a chain is, the higher likely it will be broken,
does not occur in our LSE-based encoding,
but instead the CFA modules tend to get excited,
with a very smaller number of samples in which all CFA modules functioning correcly.

\begin{figure}[!tbp]
	\centering
	\begin{minipage}{.49\linewidth}
		\includegraphics[width=1\linewidth]{figs/results/multiplier_ver2_CFA0/diff_chain_couplings/Different coupling strengths for the chain when initialized through extra chains[Jij[-2, 1] =g_min=2, J_min=-2].png}
	\end{minipage}
	\begin{minipage}{.49\linewidth}
		\includegraphics[width=1\linewidth]{figs/results/multiplier_ver2_CFA0/diff_chain_couplings/Different coupling strengths for the chain when initialized through extra chains [Jij[-1, 1] =g_min=1.333, J_min=-1].png}
	\end{minipage}
	\caption{\label{fig: diff_couplings} Different coupling strengths
	for the chain when the multiplier Hamiltonian is initialized through extra chains.}
\end{figure}

\subsection*{Excitation of CFAs and that of chains}
To examine the excitation of CFAs, we check the number of excited samples for each CFA,
how many samples out of the total 1000 samples have the specific CFA been excited,
and the starting energy from which the specific CFA got excited
and that starting energy for each chains,
which are shown in Fig \ref{fig: CFA_excitations} and Fig \ref{fig: starting_excitation_energy}.
In Fig \ref{fig: CFA_excitations}, each square represents a CFA in the multiplier circuit,
the darker it is, the higher probability it gets excited;
In Fig \ref{fig: starting_excitation_energy}, the left is for CFA excitations and the right is for chain excitations,
the lighter the squre is, the lower energy it gets excited from.

\begin{figure}[!tbp]
	\begin{minipage}{.4\linewidth}
		\centering
		\includegraphics[width=.8\linewidth]{figs/results/improved_CFA1/physical/8-8bit_factoring/input_by_chain/FW20us_factoring_47477_with_8-8bit_of_CFA_1_to_energy12.167_(201, 197, 47477)_cfhs_excitations.png}
		\caption{The number of CFA excitations}
		\label{fig: CFA_excitations}
	\end{minipage}
	\begin{minipage}{.58\linewidth}
		\centering
		\includegraphics[width=.75\linewidth]{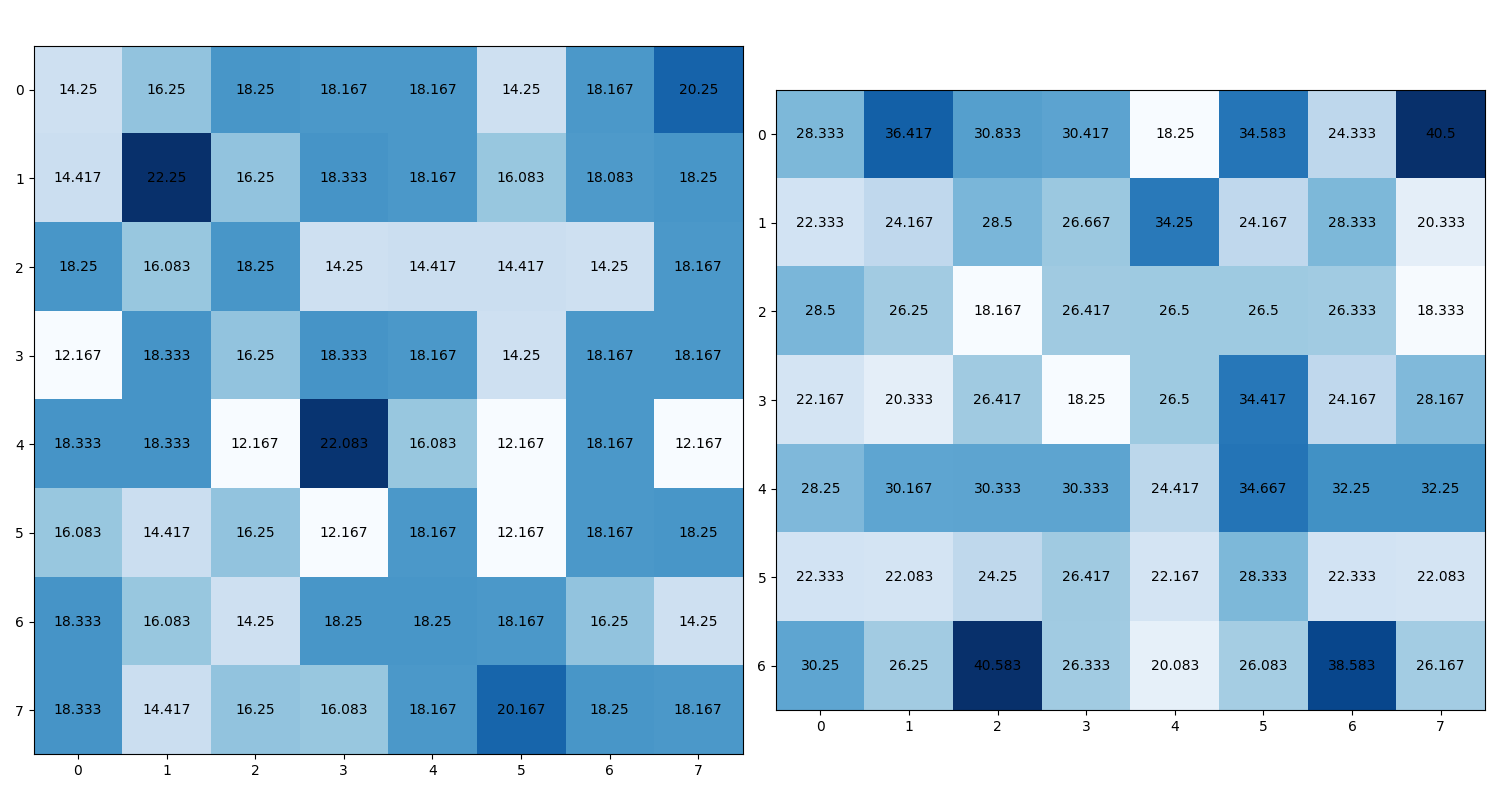}
		\caption{The starting energy that CFA gets excited and that for chains}
		\label{fig: starting_excitation_energy}
	\end{minipage}
\end{figure}

\subsection*{The symmetry of embedding}
For D-Wave Advantage system 4.1, the same penalty function,
if placed differently, 
would cause different QA performance.
Figure \ref{fig: CFA0_with_a_symmetry_embedding}, as an example,
demonstrates this performance difference
of symmetry embeddings,
by exchanging the placement of node 2 and 3
and that of node 4 and 5 of the CFA encoding of Figure \ref{fig: CFA0_encoding}.
This performance enhancement extends to solving PF problems,
whose results are shown in Figure \ref{fig: a_symmetry_embedding_small} 
and Figure \ref{fig: a_symmetry_embedding_large}. 
Therfore, the symmetry of embedding is important
for revealing the best performance out of annealers.
Although we tried to average out the performance difference
caused by the symmetry of embedding,
we haven't found a way to increase the success probability of QA to find solutions of PFs
into a higher level than the best success probability 
produced from single embedding.
What causes this performance difference
needs to be further studied.

\begin{figure}[!tbp]
	\begin{minipage}{.5\linewidth}
		\includegraphics[width=1\linewidth]{figs/results/multiplier_ver2_CFA0_with_symmetry_embeddings/Compare CFA0 with embeddings-ChainMap({}) VS ChainMap({2-3, 3-2}, {4-5, 5-4})range(3, 6).png}
	\end{minipage}
	\begin{minipage}{.5\linewidth}
		\includegraphics[width=1\linewidth]{figs/results/multiplier_ver2_CFA0_with_symmetry_embeddings/Compare CFA0 with embeddings- ChainMap({}) VS ChainMap({2-3, 3-2}, {4-5, 5-4})-BIS.png}
	\end{minipage}
	\caption{\label{fig: a_symmetry_embedding_small} The CFA with a symmetry embedding 
	for factoring $5+5, 6+6$ bit integers}
\end{figure}

\begin{figure}[!tbp]
	\includegraphics[width=1\linewidth]{figs/results/multiplier_ver2_CFA0_with_symmetry_embeddings/REVERS~1}
	\caption{\label{fig: a_symmetry_embedding_large} The CFA with a symmetry embedding 
	for factoring $8+8, ...,  14+8$ bit integers}
\end{figure}

\begin{table}[!tbp]
\scriptsize
	\centering
	\begin{tabular}{|l|r|ccc|ccc|c|}
	\toprule
	\multirow{2}{*}{size} & $P= A\times B$  &
	\multicolumn{3}{c}{Forward (+ pause)} & \multicolumn{3}{c}{Reverse (+ pause)} & 
	\multirow{2}{*}{\#$solved(P_F=0)$} \\
							&			 			 & 							
	$S_p$ & $min(P_F)$ & \#$solved$   & $S_p$ & $min(P_F)$ & \#$solved$  & \\
	\midrule
	\multirow{2}{*}{12*8} 
	&$378227= 2113 \times179$ &0.45 &4 &1   &0.51 &0 &15   &5    \\
	&$3739317= 2089\times 179$  &0.45 &2	&1   &0.49 &0 &4    &2    \\
	\midrule
	\multirow{1}{*}{13*8} 
	&$7476837= 4177\times 179$  &0.44 &4	&2   &0.51 &0 &133  &15   \\
	\midrule
	\multirow{1}{*}{14*8} 
	&$14808677= 8273\times 179$  &0.45 &4	&1   &0.5  &4 &8    &0   \\
	\bottomrule
	\end{tabular}
	\caption{\label{tab: large_factoring2} PF results using the CFA penalty function 
	,
	with input $P$ imposed by D-Wave API, {\it fix\_variables()}
	and with QA assisted by thermal relaxation.}

	\begin{tabular}{|l|r|c|c|}
	\toprule
	\multirow{2}{*}{size} & $P\Rightarrow A\times B$  &energy spectrum & distance in terms of \\
	& & Forward$\to$ Reverse & Qubit flips, CFA flips\\
	\midrule
	\multirow{2}{*}{12*8} 
	&$378227= 2113 \times179$ &
	\includegraphics[width=.3\linewidth]{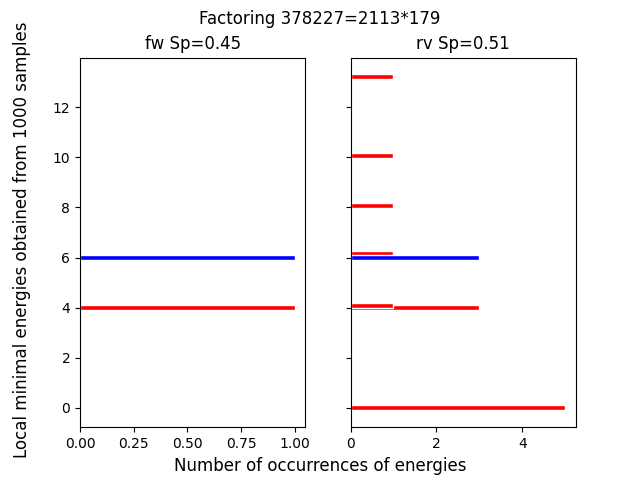} & 
	\includegraphics[width=.3\linewidth]{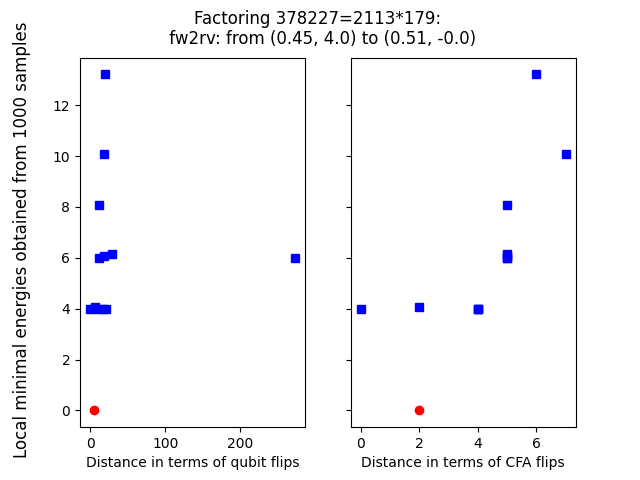}	 \\
	&$3739317= 2089\times 179$  &
	\includegraphics[width=.3\linewidth]{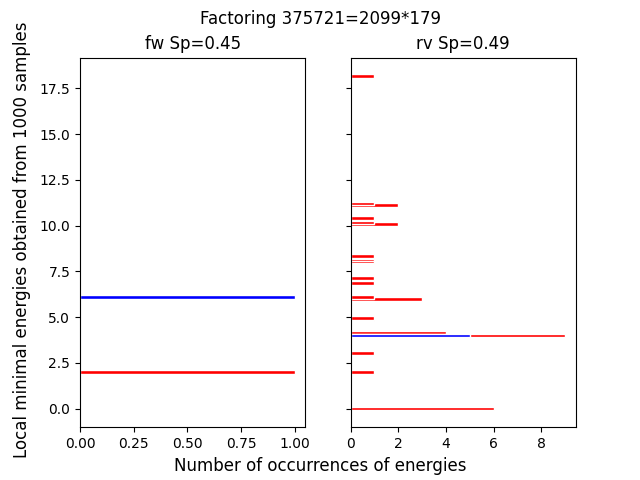}&
	\includegraphics[width=.3\linewidth]{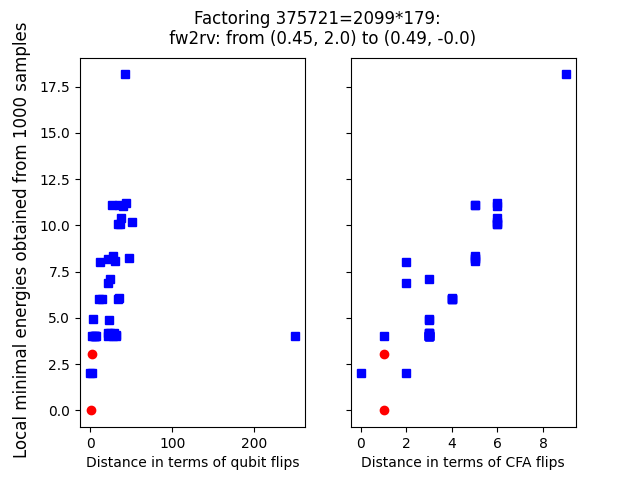}\\
	\midrule
	\multirow{1}{*}{13*8} 
	&$7476837= 4177\times 179$  &
	\includegraphics[width=.3\linewidth]{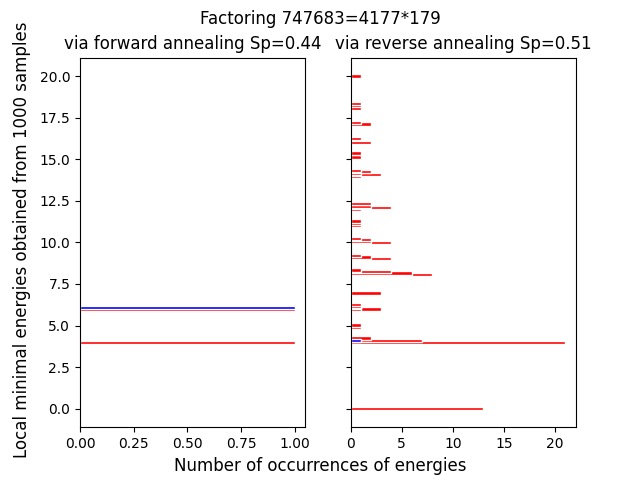}&
	\includegraphics[width=.3\linewidth]{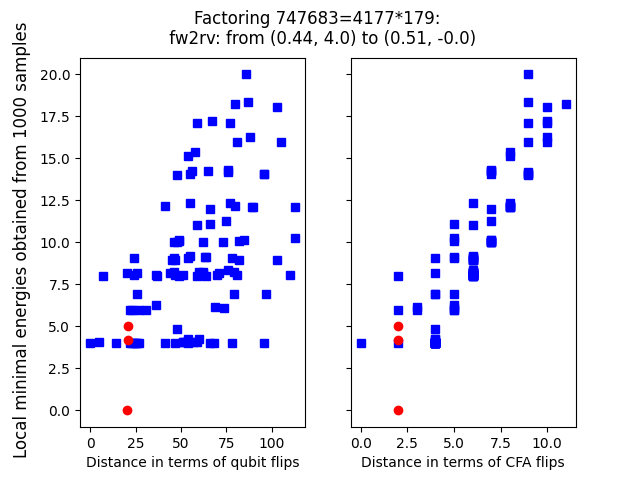}\\
	\midrule
	\multirow{1}{*}{14*8} 
	&$14808677= 8273\times 179$  &
	\includegraphics[width=.3\linewidth]{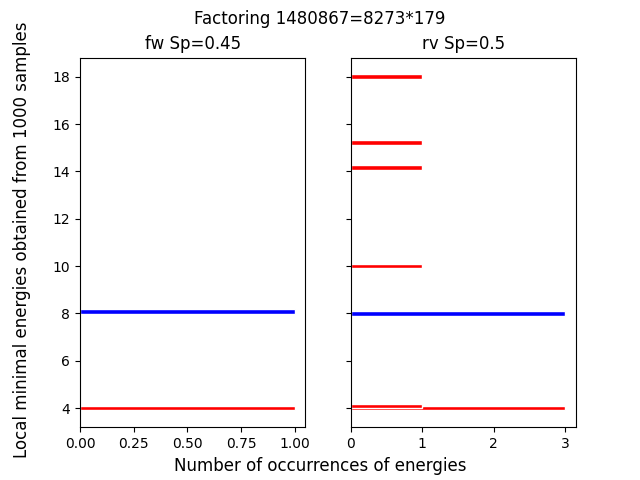}&
	\includegraphics[width=.3\linewidth]{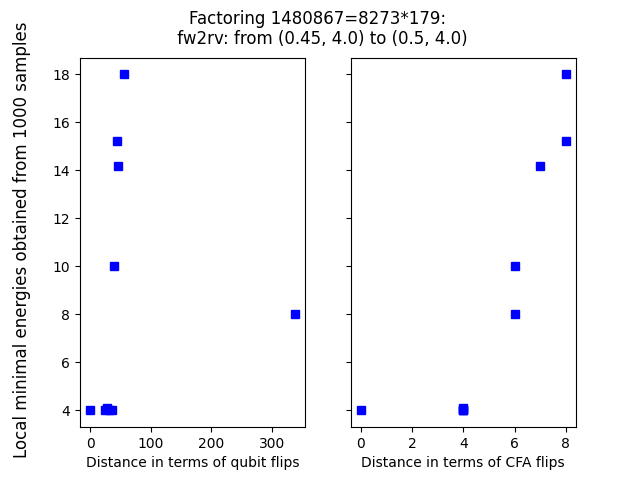}\\
	\bottomrule
	\end{tabular}
	\caption{\label{tab: large_factoring_distribution} 
	From forward to reverse of Figure \ref{tab: large_factoring},
	the changed energy distribution of both truth samples and one one false sample of lowest energy,
	and the moved Hamming distance in the unit of qubit flips (or CFA flips).
	}
\end{table}
}

\ignore{
\section*{Iterative reverse annealing: some insights}

The choice of values for both pause time and the moment when the pause is triggered are heavily correlated. In particular, for reverse annealing we noticed that:

\begin{itemize}
    \item Short pauses are effective when performed at early reversing points, if the initial state is highly excited; in the alternative when the pause is performed at a late reversing point if the starting point energy is close to zero.
    \item Long pauses are effective
\end{itemize}

\section*{Iterative reverse annealing: Jingwen original}
An important observation obtained in the previous section
is that it is quite easy for reverse annealing enhanced by thermal fluctuations
to reach groundstate from a good initial state, 
that in a quite close distance to groundstate and of quite low energy,
since the close distance can be spanned
by increasing the length of pause a little at relatively late reversion points.
Implicitly, it would also be possible for reverse annealing enhanced by thermal fluctuations
to relax an highly-excited minima in solving bigger problems,
which is quite far from groundstate, down to groundstate,
if this highly-excited minima can be gradually relaxed to such a good initial state.
With this movitation, we follow the iterative schema
and propose an iterative reverse annealing for factoring integers of 12+8 bits and even bigger.

The reverse annealing in each iteration is enhanced by thermal fluctuations, 
with the aim of approaching a lower-energy state.
The lower-energy state is assumed to be closer to groundstate,
as well as its existing lower-energy search space.
Therefore, it can be candidate for the reverse annealing in each iteration.
The risk of this assumption being broken, 
that the chosen lowest-energy state even farther from groundstate,
is taken into consideration by permitting early reversion points
$S_p\in[0.46, 0.33]$ or long pause to escape from such a worse state.

For each reverse annealing, a set of pause length $T_p \in \{1, 10, 30, 50, 100\}\mu s|T_a=20\mu s$ 
are prepared to choose for saving unnecessary QuPU time in each stage.
In the sense, short pauses can drive the system to move a very long distance 
by reverse annealing at early annealing points for highly-excited initial states
or can relax the sytem to groundstate directly by reverse annealing at late annealing points
for low-energy initial states;
long pauses can also drive the system to moves a relatively long distance
by reverse annealing at middle and late annealing points for low-energy initial states,
resulting in a state to closer groundstate or even groundstate.
Besides, in each stage different pause lengths represent moves of different magnituide,
whose combinations are assumed to able to finally consistitue a long search path to groundstate,
making the alogrithm more flexiable.
The $T_p$ in each iteration is chosen from the set in a sort of magnituide,
until a lower-energy state (i.e., the minima out of chosen $S_p$ region) is reached.
% The impact of short pauses on reaching lower-energy states 
% is speculated to disappear as the initial state's energy decreases
% and to reoccur when the initial state is very close to groundstate.
% Therefore, this selection of $T_p$ in a sort of magnituide is assumed able
% to save QuPU time as much as possible.

Last but not least, considering both the starting state of the algorithm when solving big problems,
which is obtained by pure forward annelaing, being highly excited and  
the potential limitation of moves drivable by the chosen pause set, 
we perimt relatively high-energy states, not the lowest-energy state, 
out of the lower-energy search space in begining iterations
to assist in exploring lower-energy state,
postphoning the reverse annealing of the lowest-energy state,
which may be still far from groundstate.
Through these high-energy states, which are assumed closer to groundstate 
than the previous states of the same energy level,
the reached lower-energy state is assumed also capable to appproach to groundstate further,
relative to the lowest-energy state obtained so far.
% More importantly, its required pause may be shorter than through low-energy states.

This choice of initial states in each iteration makes the algorithm
behavor like Breadth-First-Search (BFS). 
Correspondingly, the size of the lower-energy space in each iteration
determines the efficiency of this algorithm,
in terms of the number of required runs of reverse annealing to find groundstate.
Another important factor that determines this efficiency
is how each iteration contributes in approaching groundstate,
constructively or destructively, and how much.
If it is constructive, with the present parameter setting of $T_p$, 
the converge to groundstate would be fast; 
otherwise, extra iterations are required to recover the destructive iteration,
making the algorithm less efficient and costing much QuPU time.

We test this algorithm on DWave Advantage system 4.1 for factoring a number of 20 bits, 22 bits, 24 bits,
using a 12bit $\times$8bit, 14bit$\times$8bit and 16bit$\times$8bit encoded multiplier.
% from a improved CFA penalty function respectively,
% together with the initialization via flux bias.
% This improved CFA penalty function is generated by minimizing its number of first excited states
% and verified experimentally to increase the success probability of QA remain ground state.
% Furthermore, it features less energy levels, which is expected to simplify the analysis of
% the energy-level transitions in IRV.
The successful search path to reach groundstate for each problem instance
is presented in Table \ref{tab: IRV},
demonstrating that IRV is effective in reaching the ground state
from a exicited state very far away by gradually approaching it.
Moreover, this IRV turns out able to find the groundstate for a bigger problem,
factoring 4,111,631 of 22 bits, which is hard for single-iteration RV even with $600\mu s$ pause.
% as shown by a comparison of results of IRV and of RV in Table \ref{tab: IRV} and Table \ref{tab: RV}.

However, in the case of factoring 16,445,771, four iterations
turns out make the system get stuck in a minima state with energy equal to four,
which cannot be escaped with a pause of $T_p=100\mu s$.
For resolving this situation, we update the set of pause length 
with long pause, e.g., $T_p\in\{100, 200\}\mu s$, for each iteration
to trigger large moves;
on the other hand, we also expect these large moves 
to improve the efficiency of iterative reverse annealing.
Due to possible lager moves than the previous version of IRV, 
the lowest-energy state could be chosen
for the initial state of reverse annealing ealier.
Note that $T_p=1\mu s$ can be reserved for reversing annealing 
from a highly-excited state due to possible large moves.
The experimental results shown in Table \ref{tab: tab: more_effient_IRV}
demonstrate the improvement of the efficiency of this variant IRV,
reaching groundstate for factoring 2, 055, 941 of 13+8 bits
and 4, 111, 631 of 15+8 bits with only two iterations.
However, for factoring 8, 219, 999 of 16+8 bits,
the second and third iteration reverse annealing
seems contribute in approaching groundstate destructively,
with the contribution of the first iteration removed.
This is because the choice of the initial state of reverse annealing
is based on the lowest-energy state, 
which cannot always guarantee the closest state to groundstate,
bottleneck of the current algorithm.
The location of the closest state to groundstate 
out of reversion region of reverse annealing against its energy 
will be explored for different pause lengths in the future,
to further improve the efficiency of our algorithm.
}
